# Supplementary material for: Tensor hypercontraction for self-consistent vertex corrected GW with static and dynamic screening; applications to molecules and solids with superexchange
Source: arXiv:2412.18829 source file (2024-12-25)
Supplement: Supplementary file 1 [file SI.pdf]

# Tensor hypercontraction for self-consistent vertex corrected GW with static and dynamic screening; applications to molecules and solids with superexchange

Pavel Pokhilko,[1] Chia-Nan Yeh,[2] Miguel A. Morales,[2] and Dominika Zgid[1,3]

[1]*Department of Chemistry, University of Michigan, Ann Arbor, Michigan 48109, USA*
[2]*Center for Computational Quantum Physics, Flatiron Institute, New York, New York 10010, USA*
[3]*Department of Physics, University of Michigan, Ann Arbor, Michigan 48109, USA*

TABLE S1: Contributions of 2p oxygen's AOs to SA-NOs of broken-symmetry solutions for $[Fe_2OCl_6]^{2-}$. Both occupancies of SA-NOs and coefficients are shown.

| | | | |
|---|---|---|---|
| UHF occ | 0.906 | 0.927 | 0.929 |
| $p_x$ | -0.062 | -0.170 | -0.001 |
| $p_y$ | 0.004 | 0.000 | -0.176 |
| $p_z$ | -0.194 | 0.054 | -0.004 |
| GW occ | 0.825 | 0.850 | 0.851 |
| $p_x$ | -0.081 | -0.247 | -0.021 |
| $p_y$ | 0.012 | 0.019 | -0.260 |
| $p_z$ | -0.251 | 0.080 | -0.005 |
| GWSOX occ | 0.859 | 0.887 | 0.889 |
| $p_x$ | -0.070 | -0.201 | -0.003 |
| $p_y$ | 0.006 | 0.002 | -0.210 |
| $p_z$ | -0.219 | 0.065 | -0.005 |

TABLE S2: Neel temperature estimates ($J_2$ units and K) for NiO evaluated with different methods.

| $n$ | UHF | | GW | | GWSOX | |
|---|---|---|---|---|---|---|
| | $g_n(J_1/J_2,1)$ | $g_n(J_1,J_2)$ | $g_n(J_1/J_2,1)$ | $g_n(J_1,J_2)$ | $g_n(J_1/J_2,1)$ | $g_n(J_1,J_2)$ |
| 2 | 1.837 | 107 | 1.994 | 309 | 1.830 | 187 |
| 3 | 1.581 | 92 | 1.856 | 288 | 1.568 | 160 |
| 4 | 0.852 | 49 | 1.544 | 240 | 0.790 | 81 |
| 5 | 1.721 | 100 | 1.215 | 188 | 1.732 | 177 |
| 6 | 1.974 | 115 | 1.856 | 288 | 1.975 | 202 |
| 7 | 2.020 | 117 | 2.050 | 318 | 2.017 | 206 |
| 8 | 1.956 | 113 | 2.096 | 325 | 1.946 | 199 |
| 9 | 1.800 | 104 | 2.076 | 322 | 1.779 | 182 |
| 10 | 1.573 | 91 | 1.999 | 310 | 1.622 | 166 |

| $n$ | GWSOSEXstat | | GWSOSEXdyn | | G3W2stat | |
|---|---|---|---|---|---|---|
| | $g_n(J_1/J_2,1)$ | $g_n(J_1,J_2)$ | $g_n(J_1/J_2,1)$ | $g_n(J_1,J_2)$ | $g_n(J_1/J_2,1)$ | $g_n(J_1,J_2)$ |
| 2 | 1.944 | 261 | 1.950 | 257 | 1.985 | 306 |
| 3 | 1.771 | 238 | 1.780 | 235 | 1.841 | 284 |
| 4 | 1.381 | 185 | 1.401 | 185 | 1.517 | 234 |
| 5 | 1.466 | 197 | 1.445 | 191 | 1.274 | 196 |
| 6 | 1.914 | 257 | 1.909 | 252 | 1.868 | 288 |
| 7 | 2.054 | 276 | 2.054 | 271 | 2.052 | 316 |
| 8 | 2.066 | 277 | 2.070 | 273 | 2.092 | 322 |
| 9 | 2.014 | 270 | 2.022 | 267 | 2.067 | 319 |
| 10 | 1.886 | 253 | 1.901 | 251 | 1.981 | 306 |

| $n$ | GW2SOSEXstat | | GW2SOSEXdyn | |
|---|---|---|---|---|
| | $g_n(J_1/J_2,1)$ | $g_n(J_1,J_2)$ | $g_n(J_1/J_2,1)$ | $g_n(J_1,J_2)$ |
| 2 | 2.047 | 392 | | |
| 3 | 1.943 | 372 | | |
| 4 | 1.692 | 324 | | |
| 5 | 0.924 | 177 | | |
| 6 | 1.760 | 337 | | |
| 7 | 2.029 | 389 | | |
| 8 | 2.114 | 405 | | |
| 9 | 2.124 | 407 | | |
| 10 | 2.083 | 399 | | |

TABLE S3: Neel temperature estimates ($J_2$ units and K) for MnO evaluated with different methods.

| $n$ | UHF | | GW | | GWSOX | |
|---|---|---|---|---|---|---|
| | $g_n(J_1/J_2,1)$ | $g_n(J_1,J_2)$ | $g_n(J_1/J_2,1)$ | $g_n(J_1,J_2)$ | $g_n(J_1/J_2,1)$ | $g_n(J_1,J_2)$ |
| 2 | 58.098 | 128 | 54.751 | 364 | 61.745 | 242 |
| 3 | 54.578 | 120 | 51.446 | 342 | 57.979 | 227 |
| 4 | 53.205 | 117 | 50.107 | 333 | 56.546 | 222 |
| 5 | 51.940 | 114 | 49.106 | 326 | 55.042 | 216 |
| 6 | 51.511 | 113 | 48.627 | 323 | 54.642 | 214 |
| 7 | 51.084 | 113 | 48.231 | 320 | 54.181 | 213 |
| 8 | 50.765 | 112 | 47.935 | 318 | 53.838 | 211 |
| 9 | 50.518 | 111 | 47.706 | 317 | 53.573 | 210 |
| 10 | 50.322 | 111 | 47.523 | 316 | 53.361 | 209 |
| | GWSOSEXstat | | GWSOSEXdyn | | G3W2stat | |
| | $g_n(J_1/J_2,1)$ | $g_n(J_1,J_2)$ | $g_n(J_1/J_2,1)$ | $g_n(J_1,J_2)$ | $g_n(J_1/J_2,1)$ | $g_n(J_1,J_2)$ |
| 2 | 58.332 | 321 | 56.303 | 314 | 56.316 | 362 |
| 3 | 54.796 | 301 | 52.899 | 295 | 52.912 | 340 |
| 4 | 53.420 | 294 | 51.547 | 287 | 51.560 | 332 |
| 5 | 52.139 | 287 | 50.418 | 281 | 50.429 | 325 |
| 6 | 51.711 | 284 | 49.965 | 278 | 49.977 | 322 |
| 7 | 51.282 | 282 | 49.555 | 276 | 49.566 | 319 |
| 8 | 50.962 | 280 | 49.248 | 274 | 49.260 | 317 |
| 9 | 50.714 | 279 | 49.011 | 273 | 49.022 | 315 |
| 10 | 50.516 | 278 | 48.821 | 272 | 48.832 | 314 |
| | GW2SOSEXstat | | GW2SOSEXdyn | | | |
| | $g_n(J_1/J_2,1)$ | $g_n(J_1,J_2)$ | $g_n(J_1/J_2,1)$ | $g_n(J_1,J_2)$ | | |
| 2 | 55.634 | 419 | | | | |
| 3 | 52.273 | 394 | | | | |
| 4 | 50.928 | 384 | | | | |
| 5 | 49.852 | 376 | | | | |
| 6 | 49.389 | 372 | | | | |
| 7 | 48.985 | 369 | | | | |
| 8 | 48.683 | 367 | | | | |
| 9 | 48.449 | 365 | | | | |
| 10 | 48.262 | 364 | | | | |
